# Supplementary material for: Adjusting for Participation Bias in Case-Control Genetic Association Studies for Rare Diseases
Source: arXiv:2407.08382 ancillary file (2024-07-11)
Supplement: Supplementary file 1 [file FSWEL_arxiv_supp.pdf]

# Supplementary Material for Adjusting for Participation Bias in Case-Control Genetic Association Studies for Rare Diseases

Le Wang [*] Zhengbang Li[*] Ben Fitzpatrick Clarice Weinberg Jinbo Chen

In this section, we derive the expectation of the likelihood score function of the missingness model (1) in the manuscript conditional on the observed data $\boldsymbol{b}_i = (Y_i, \boldsymbol{X}_i, G_i^f, R = 0)$ for the $i$th individual whose genotype is missing. We define $\boldsymbol{d}_i$ as a vector of all covariates and the interaction terms in the missingness model for the $i$th individual.

$$
\begin{aligned}
E\big(S_i(\boldsymbol{\alpha})|\boldsymbol{b}_i\big) &= -\,E(\boldsymbol{d}_i \mathrm{P}(R=1|Y_i,\boldsymbol{X}_i,G_i)|\boldsymbol{b}_i)\\
&= -\sum_g \boldsymbol{d}_i \mathrm{P}(R=1|Y_i,\boldsymbol{X}_i,G)\mathrm{P}(G|\boldsymbol{b}_i)\\
&= \frac{-\sum_g \boldsymbol{d}_i \mathrm{P}(R=1|Y_i,\boldsymbol{X}_i,G)\mathrm{P}(R=0|Y_i,\boldsymbol{X}_i,G,G_i^f)\mathrm{P}(G|Y_i,\boldsymbol{X}_i,G_i^f)}{\mathrm{P}(R=0|Y_i,\boldsymbol{X}_i,G_i^f)}\\
&= \frac{-\sum_g \boldsymbol{d}_i \mathrm{P}(R=1|Y_i,\boldsymbol{X}_i,G)\mathrm{P}(R=0|Y_i,\boldsymbol{X}_i,G,G_i^f)\mathrm{P}(G,\boldsymbol{X}_i,G_i^f|Y_i)}{\mathrm{P}(R=0|Y_i,\boldsymbol{X}_i,G_i^f)\sum_g \mathrm{P}(G,\boldsymbol{X}_i,G_i^f|Y_i)}\\
&= \frac{-\sum_g \boldsymbol{d}_i \mathrm{P}(R=1|Y_i,\boldsymbol{X}_i,G)\mathrm{P}(R=0|Y_i,\boldsymbol{X}_i,G,G_i^f)\mathrm{P}(G,\boldsymbol{X}_i,G_i^f|Y_i)}{\sum_g \mathrm{P}(R=0,G|Y_i,\boldsymbol{X}_i,G_i^f)\sum_g \mathrm{P}(G,\boldsymbol{X}_i,G_i^f|Y_i)}\\
&= \frac{-\sum_g \boldsymbol{d}_i \mathrm{P}(R=1|Y_i,\boldsymbol{X}_i,G)\mathrm{P}(R=0|Y_i,\boldsymbol{X}_i,G,G_i^f)\mathrm{P}(G,\boldsymbol{X}_i,G_i^f|Y_i)}{\sum_g\{\mathrm{P}(R=0|G,Y_i,\boldsymbol{X}_i,G_i^f)\mathrm{P}(G|Y_i,\boldsymbol{X}_i,G_i^f)\}\sum_g \mathrm{P}(G,\boldsymbol{X}_i,G_i^f|Y_i)}\\
&= \frac{-\sum_g \boldsymbol{d}_i \mathrm{P}(R=1|Y_i,\boldsymbol{X}_i,G)\mathrm{P}(R=0|Y_i,\boldsymbol{X}_i,G,G_i^f)\mathrm{P}(G,\boldsymbol{X}_i,G_i^f|Y_i)}{\sum_g\{\mathrm{P}(R=0|Y_i,\boldsymbol{X}_i,G,G_i^f)\frac{\mathrm{P}(G,\boldsymbol{X}_i,G_i^f|Y_i)}{\sum_g \mathrm{P}(G,\boldsymbol{X}_i,G_i^f|Y_i)}\}\sum_g \mathrm{P}(G,\boldsymbol{X}_i,G_i^f|Y_i)}\\
&= \frac{-\sum_g \boldsymbol{d}_i \mathrm{P}(R=1|Y_i,\boldsymbol{X}_i,G)\mathrm{P}(R=0|Y_i,\boldsymbol{X}_i,G,G_i^f)\mathrm{P}(G,\boldsymbol{X}_i,G_i^f|Y_i)}{\sum_g\{\mathrm{P}(R=0|Y_i,\boldsymbol{X}_i,G,G_i^f)\mathrm{P}(G,\boldsymbol{X}_i,G_i^f|Y_i)\}}
\end{aligned}
$$

Following the result of Satten and Kupper (1993) for a rare outcome to relate $\mathrm{P}(\boldsymbol{X},G,G^f|Y=1)$ and $\mathrm{P}(\boldsymbol{X},G,G^f|Y=0)$, i.e.,

$$
\mathrm{P}(\boldsymbol{X},G,G^f|Y=1) = \frac{e^{f_\beta(\boldsymbol{X},G)}\mathrm{P}(\boldsymbol{X},G,G^f|Y=0)}{\sum_x\sum_g e^{f_\beta(\boldsymbol{X},G)}\mathrm{P}(\boldsymbol{X},G,G^f|Y=0)},
$$

[*]Two authors contributed equally to the method development.

the conditional expectation of the score function can be further derived as

$$E\big(S_i(\boldsymbol{\alpha})|\boldsymbol{b}_i\big) \approx \frac{-\sum_g \boldsymbol{d}_i \mathrm{P}(R=1|Y_i,\boldsymbol{X}_i,G)\mathrm{P}(R=0|Y_i,\boldsymbol{X}_i,G,G_i^f)e^{Y_i f_\beta(\boldsymbol{X}_i,G)}\mathrm{P}(\boldsymbol{X}_i,G,G_i^f|Y=0)}{\sum_g \mathrm{P}(R=0|Y_i,\boldsymbol{X}_i,G,G_i^f)e^{Y_i f_\beta(\boldsymbol{X}_i,G)}\mathrm{P}(\boldsymbol{X}_i,G,G_i^f|Y=0)}$$

$$=\frac{-\sum_g \boldsymbol{d}_i \mathrm{P}(R=1|Y_i,\boldsymbol{X}_i,G)\mathrm{P}(R=0|Y_i,\boldsymbol{X}_i,G)e^{Y_i f_\beta(\boldsymbol{X}_i,G)}\mathrm{P}(\boldsymbol{X}_i|G,G^f,Y=0)\mathrm{P}(G,G_i^f|Y=0)}{\sum_g \mathrm{P}(R=0|Y_i,\boldsymbol{X}_i,G)e^{Y_i f_\beta(\boldsymbol{X}_i,G)}\mathrm{P}(\boldsymbol{X}_i|G,G^f,Y=0)\mathrm{P}(G,G_i^f|Y=0)}$$

$$\approx\frac{-\sum_g \boldsymbol{d}_i \mathrm{P}(R=1|Y_i,\boldsymbol{X}_i,G)\mathrm{P}(R=0|Y_i,\boldsymbol{X}_i,G)e^{Y_i f_\beta(\boldsymbol{X}_i,G)}\mathrm{P}(\boldsymbol{X}_i|G,Y=0)\mathrm{P}_\theta(G,G_i^f)}{\sum_g \mathrm{P}(R=0|Y_i,\boldsymbol{X}_i,G)e^{Y_i f_\beta(\boldsymbol{X}_i,G)}\mathrm{P}(\boldsymbol{X}_i|G,Y=0)\mathrm{P}_\theta(G,G_i^f)}$$

Note that under the rare disease assumption, the joint distribution of an individual's genotype $G$ and family's genotype $G^f$ can be approximated by that in the full population, i.e., $\mathrm{P}(G,G^f|Y=0) \approx \mathrm{P}_\theta(G,G^f)$. Conditional on outcome $Y$, covariate $\boldsymbol{X}$, and genotype $G$, the probability of genotype availability does not depend on family member's genotype $G^f$, i.e. $\mathrm{P}(R|Y,\boldsymbol{X},G,G^f) = \mathrm{P}(R|Y,\boldsymbol{X},G)$. Given genotype $G$, the distribution of covariate $\boldsymbol{X}$ among controls does not depend on $G^f$, that is $\mathrm{P}(\boldsymbol{X}|G,G^f,Y=0) = \mathrm{P}(\boldsymbol{X}|G,Y=0)$.

In this section, we derive the asymptotic properties of the family-supplemented weighted empirical likelihood method. We obtain point estimates $(\hat{\boldsymbol{\eta}}^T, \hat{\boldsymbol{\alpha}}^T, \hat{\boldsymbol{\delta}}(\hat{\boldsymbol{\alpha}})^T)^T$ by jointly solving estimating equations (3), (4), and (5) in the manuscript. The expectations of these estimating functions, upon setting all parameters at the true values, equal zero, implying the consistency of $(\hat{\boldsymbol{\eta}}^T, \hat{\boldsymbol{\alpha}}^T, \hat{\boldsymbol{\delta}}(\hat{\boldsymbol{\alpha}})^T)^T$ under regularity conditions (Theorem 5.9 and 5.21 [1]). Let $p_1$ and $p_0$ denote the proportions of cases and controls in the sample, respectively. First we expand the estimating function for the association model about the true parameters $(\boldsymbol{\eta}^T, \boldsymbol{\delta}^T, \boldsymbol{\alpha}^T)^T$ by Taylor series

$$\begin{aligned}\mathbf{0} \approx & \frac{1}{N}\sum_{i=1}^{N}\frac{R_i}{\pi_i(\boldsymbol{\alpha})}U_i(\boldsymbol{\eta},\boldsymbol{\delta}) + \frac{1}{N}\sum_{i=1}^{N}\frac{R_i}{\pi_i(\boldsymbol{\alpha})}\frac{\partial U_i(\boldsymbol{\eta},\boldsymbol{\delta})}{\partial \boldsymbol{\eta}}(\hat{\boldsymbol{\eta}}-\boldsymbol{\eta}) \\ & + \frac{1}{N}\sum_{i=1}^{N}\left\{\frac{R_i}{\pi_i(\boldsymbol{\alpha})}\frac{\partial U_i(\boldsymbol{\eta},\boldsymbol{\delta})}{\partial \boldsymbol{\delta}}\frac{\partial \hat{\boldsymbol{\delta}}(\boldsymbol{\alpha})}{\partial \boldsymbol{\alpha}} - U_i(\boldsymbol{\eta},\boldsymbol{\delta})\frac{R_i}{\pi_i^2(\boldsymbol{\alpha})}\frac{\partial \pi_i(\boldsymbol{\alpha})}{\partial \boldsymbol{\alpha}}\right\}(\hat{\boldsymbol{\alpha}}-\boldsymbol{\alpha}) \\ & + \frac{1}{N}\sum_{i=1}^{N}\frac{R_i}{\pi_i(\boldsymbol{\alpha})}\frac{\partial U_i(\boldsymbol{\eta},\boldsymbol{\delta})}{\partial \boldsymbol{\delta}}(\hat{\boldsymbol{\delta}}(\boldsymbol{\alpha})-\boldsymbol{\delta}).\end{aligned}$$

The coefficient for $\hat{\boldsymbol{\eta}}-\boldsymbol{\eta}$ converges in probability to a constant matrix denoted by $C_1$:

$$\begin{aligned}\frac{1}{N}\sum_{i=1}^{N}\frac{R_i}{\pi_i(\boldsymbol{\alpha})}\frac{\partial U_i(\boldsymbol{\eta},\boldsymbol{\delta})}{\partial \boldsymbol{\eta}} &= \frac{1}{N}\sum_{y}\sum_{i=1}^{N_y}\frac{R_i}{\pi_i(\boldsymbol{\alpha})}\left\{\frac{\partial U_i(\boldsymbol{\eta},\boldsymbol{\delta})}{\partial \boldsymbol{\eta}}\right\} \\ &= \sum_{y}\left\{\frac{N_y}{N}\frac{1}{N_y}\sum_{i=1}^{N_y}\frac{R_i}{\pi_i(\boldsymbol{\alpha})}\left\{\frac{\partial U_i(\boldsymbol{\eta},\boldsymbol{\delta})}{\partial \boldsymbol{\eta}}\right\}\right\} \\ &\xrightarrow{P} \sum_{y} p_y E_{Y=y}\left\{\frac{\partial U_i(\boldsymbol{\eta},\boldsymbol{\delta})}{\partial \boldsymbol{\eta}}\right\} \\ &= E_{\{Y,\boldsymbol{X},G\}}\left\{\frac{\partial U_i(\boldsymbol{\eta},\boldsymbol{\delta})}{\partial \boldsymbol{\eta}}\right\} = C_1,\end{aligned}$$

where expectation $E_{Y=y}(\cdot)$ is taken with respect to the joint distribution of $(\boldsymbol{X}, G)$ within cases or controls, i.e., $\mathrm{P}(\boldsymbol{X}, G|Y=y)$, and $E_{\{Y,\boldsymbol{X},G\}}(\cdot)$ is taken with respect to probability $\mathrm{P}(Y, \boldsymbol{X}, G)$ in the full case-control sample. Note that cases and controls are calculated separately in the case-control sample under the association model. Similarly, the coefficients for $\hat{\boldsymbol{\alpha}}-\boldsymbol{\alpha}$ and $\hat{\boldsymbol{\delta}}(\boldsymbol{\alpha})-\boldsymbol{\delta}$ converge in probability to two constant matrices $C_2$ and $C_3$, respectively:

$$\frac{1}{N}\sum_{i=1}^{N}\frac{R_i}{\pi_i(\boldsymbol{\alpha})}\frac{\partial U_i(\boldsymbol{\eta},\boldsymbol{\delta})}{\partial \boldsymbol{\delta}}\frac{\partial \hat{\boldsymbol{\delta}}(\boldsymbol{\alpha})}{\partial \boldsymbol{\alpha}} \xrightarrow{P} E_{\{Y,\boldsymbol{X},G\}}\left\{\frac{\partial U_i(\boldsymbol{\eta},\boldsymbol{\delta})}{\partial \boldsymbol{\delta}}\frac{\partial \hat{\boldsymbol{\delta}}(\boldsymbol{\alpha})}{\partial \boldsymbol{\alpha}}\right\} = C_{21},$$

$$\begin{aligned}\frac{1}{N}\sum_{i=1}^{N}U_i(\boldsymbol{\eta},\boldsymbol{\delta})\frac{R_i}{\pi_i^2(\boldsymbol{\alpha})}\frac{\partial \pi_i(\boldsymbol{\alpha})}{\partial \boldsymbol{\alpha}} &\xrightarrow{P} E_{\{Y,\boldsymbol{X},G\}}\left\{U_i(\boldsymbol{\eta},\boldsymbol{\delta})\frac{1}{\pi_i(\boldsymbol{\alpha})}\frac{\partial \pi_i(\boldsymbol{\alpha})}{\partial \boldsymbol{\alpha}}\right\} \\ &= E_{\{Y,\boldsymbol{X},G\}}\left\{U_i(\boldsymbol{\eta},\boldsymbol{\delta})\frac{\partial \log \pi_i(\boldsymbol{\alpha})}{\partial \boldsymbol{\alpha}}\right\} = C_{22},\end{aligned}$$

$$\frac{1}{N}\sum_{i=1}^{N}\frac{R_i}{\pi_i(\boldsymbol{\alpha})}\frac{\partial U_i(\boldsymbol{\eta},\boldsymbol{\delta})}{\partial \boldsymbol{\delta}} \xrightarrow{P} E_{\{Y,\boldsymbol{X},G\}}\left\{\frac{\partial U_i(\boldsymbol{\eta},\boldsymbol{\delta})}{\partial \boldsymbol{\delta}}\right\} = C_3,$$

where we define $C_2 = C_{21} - C_{22}$. Therefore, the estimating function for the association model can be written as

$$\mathbf{0} = \frac{1}{N}\sum_{i=1}^{N} \frac{R_i}{\pi_i(\boldsymbol{\alpha})} U_i(\boldsymbol{\eta}, \boldsymbol{\delta}) + C_1(\hat{\boldsymbol{\eta}} - \boldsymbol{\eta}) + C_2(\hat{\boldsymbol{\alpha}} - \boldsymbol{\alpha}) + C_3(\hat{\boldsymbol{\delta}}(\boldsymbol{\alpha}) - \boldsymbol{\delta}). \tag{1}$$

Then we apply Taylor expansion to the estimating function for the missingness model about the true parameters $(\boldsymbol{\eta}^T, \boldsymbol{\delta}^T, \boldsymbol{\alpha}^T)^T$, i.e.,

$$\begin{aligned}\mathbf{0} \approxeq & \frac{1}{N}\sum_{i=1}^{N} U_i^m(\boldsymbol{\alpha}, \boldsymbol{\delta}, \boldsymbol{\eta}) + \frac{1}{N}\sum_{i=1}^{N} \frac{\partial U_i^m(\boldsymbol{\alpha}, \boldsymbol{\delta}, \boldsymbol{\eta})}{\partial \boldsymbol{\eta}} (\hat{\boldsymbol{\eta}} - \boldsymbol{\eta}) \\ & + \frac{1}{N}\sum_{i=1}^{N} \left( \frac{\partial U_i^m(\boldsymbol{\alpha}, \boldsymbol{\delta}, \boldsymbol{\eta})}{\partial \boldsymbol{\alpha}} + \frac{\partial U_i^m(\boldsymbol{\alpha}, \boldsymbol{\delta}, \boldsymbol{\eta})}{\partial \boldsymbol{\delta}} \frac{\partial \hat{\boldsymbol{\delta}}(\boldsymbol{\alpha})}{\partial \boldsymbol{\alpha}} \right) (\hat{\boldsymbol{\alpha}} - \boldsymbol{\alpha}) \\ & + \frac{1}{N}\sum_{i=1}^{N} \frac{\partial U_i^m(\boldsymbol{\alpha}, \boldsymbol{\delta}, \boldsymbol{\eta})}{\partial \boldsymbol{\delta}} (\hat{\boldsymbol{\delta}}(\boldsymbol{\alpha}) - \boldsymbol{\delta}),\end{aligned}$$

and the coefficients for $\hat{\boldsymbol{\eta}} - \boldsymbol{\eta}$, $\hat{\boldsymbol{\alpha}} - \boldsymbol{\alpha}$ and $\hat{\boldsymbol{\delta}}(\boldsymbol{\alpha}) - \boldsymbol{\delta}$ converge in probability to the constant matrices below

$$\frac{1}{N}\sum_{i=1}^{N} \frac{\partial U_i^m(\boldsymbol{\alpha}, \boldsymbol{\delta}, \boldsymbol{\eta})}{\partial \boldsymbol{\eta}} \xrightarrow{P} E_{\{Y, \boldsymbol{X}, G, G^f\}} \left\{ \frac{\partial U_i^m(\boldsymbol{\alpha}, \boldsymbol{\delta}, \boldsymbol{\eta})}{\partial \boldsymbol{\eta}} \right\} = D_1,$$

$$\frac{1}{N}\sum_{i=1}^{N} \frac{\partial U_i^m(\boldsymbol{\alpha}, \boldsymbol{\delta}, \boldsymbol{\eta})}{\partial \boldsymbol{\alpha}} \xrightarrow{P} E_{\{Y, \boldsymbol{X}, G, G^f\}} \left\{ \frac{\partial U_i^m(\boldsymbol{\alpha}, \boldsymbol{\delta}, \boldsymbol{\eta})}{\partial \boldsymbol{\alpha}} \right\} = D_{21},$$

$$\frac{1}{N}\sum_{i=1}^{N} \frac{\partial U_i^m(\boldsymbol{\alpha}, \boldsymbol{\delta}, \boldsymbol{\eta})}{\partial \boldsymbol{\delta}} \frac{\partial \hat{\boldsymbol{\delta}}(\boldsymbol{\alpha})}{\partial \boldsymbol{\alpha}} \xrightarrow{P} E_{\{Y, \boldsymbol{X}, G, G^f\}} \left\{ \frac{\partial U_i^m(\boldsymbol{\alpha}, \boldsymbol{\delta}, \boldsymbol{\eta})}{\partial \boldsymbol{\delta}} \frac{\partial \hat{\boldsymbol{\delta}}(\boldsymbol{\alpha})}{\partial \boldsymbol{\alpha}} \right\} = D_{22},$$

$$\frac{1}{N}\sum_{i=1}^{N} \frac{\partial U_i^m(\boldsymbol{\alpha}, \boldsymbol{\delta}, \boldsymbol{\eta})}{\partial \boldsymbol{\delta}} \xrightarrow{P} E_{\{Y, \boldsymbol{X}, G, G^f\}} \left\{ \frac{\partial U_i^m(\boldsymbol{\alpha}, \boldsymbol{\delta}, \boldsymbol{\eta})}{\partial \boldsymbol{\delta}} \right\} = D_3,$$

where we define $D_2 = D_{21} + D_{22}$ and $E_{\{Y, \boldsymbol{X}, G, G^f\}}(\cdot)$ are taken with respect to the joint distribution $\mathrm{P}(Y, X, G, G^f)$ in the full sample. Hence, the estimating function for the missingness model can be written as

$$\mathbf{0} = \frac{1}{N}\sum_{i=1}^{N} U_i^m(\boldsymbol{\alpha}, \boldsymbol{\delta}, \boldsymbol{\eta}) + D_1(\hat{\boldsymbol{\eta}} - \boldsymbol{\eta}) + D_2(\hat{\boldsymbol{\alpha}} - \boldsymbol{\alpha}) + D_3(\hat{\boldsymbol{\delta}}(\boldsymbol{\alpha}) - \boldsymbol{\delta}). \tag{2}$$

Then we define $c_i = \mathrm{P}(R = 1 | Y = 0, \boldsymbol{x}_i, g_i)\mathrm{P}(G = g | Y = 0)$ and re-write the nonparametric estimator for each element $\delta_{\boldsymbol{x}g}$ in the vector $\boldsymbol{\delta}$ as

$$\hat{\delta}_{\boldsymbol{x}g}(\boldsymbol{\alpha}) = \frac{1}{N_0}\sum_{i=1}^{N_0} \frac{I(R_i = 1, \boldsymbol{X}_i = \boldsymbol{x}, G_i = g)}{\mathrm{P}(R = 1 | Y = 0, \boldsymbol{x}_i, g_i) \frac{1}{N_0} \sum_{i=1}^{N_0} \frac{I(R_i = 1, G_i = g)}{\mathrm{P}(R = 1 | Y = 0, \boldsymbol{x}_i, g_i)}},$$

where

$$\frac{1}{N_0}\sum_{i=1}^{N_0}\frac{I(R_i=1,G_i=g)}{\mathrm{P}(R=1|Y=0,\boldsymbol{x}_i,g_i)}\xrightarrow{P}E\left\{I(G_i=g)|Y=0\right\}=\mathrm{P}(G=g|Y=0);$$

therefore,

$$\hat{\delta}_{\boldsymbol{x}g}(\boldsymbol{\alpha})-\delta_{\boldsymbol{x}g}(\boldsymbol{\alpha})=\frac{1}{N_0}\sum_{i=1}^{N_0}\left\{\frac{I(R_i=1,\boldsymbol{X}_i=x,G_i=g)}{c_i}-\delta_{\boldsymbol{x}g}\right\}=\frac{1}{N_0}\sum_{i=1}^{N_0}f_i^{xg},$$

where $c_i=\mathrm{P}(R=1|Y=0,\boldsymbol{x}_i,g_i)\mathrm{P}(G=g|Y=0)$. Let $\boldsymbol{f}_i$ denote the vector of $\{f_i^{\boldsymbol{x}g},\boldsymbol{x}=\boldsymbol{x}^1,\boldsymbol{x}^2,...,\boldsymbol{x}^{J-1}$ and $g=0,1,2\}$ and thus the influence function for the nuisance parameter $\boldsymbol{\delta}$ is

$$\hat{\boldsymbol{\delta}}(\boldsymbol{\alpha})-\boldsymbol{\delta}=\frac{1}{N_0}\sum_{i=1}^{N_0}\boldsymbol{f}_i. \tag{3}$$

Then we define the $i$th subject's contribution to the estimating functions of the association and missingness models as $\boldsymbol{a}_i=\frac{R_i}{\pi_i(\boldsymbol{\alpha})}U_i(\boldsymbol{\eta},\boldsymbol{\delta})$ and $\boldsymbol{b}_i=U_i^m(\boldsymbol{\alpha},\boldsymbol{\delta},\boldsymbol{\eta})$, and define matrix

$$M=\begin{bmatrix}C_1 & C_2\\ D_1 & D_2\end{bmatrix}.$$

Then we substitute the expression of $\hat{\boldsymbol{\delta}}(\boldsymbol{\alpha})-\boldsymbol{\delta}$ in equation (3) into equation (1) and equation (2), i.e.,

$$M\begin{bmatrix}\hat{\boldsymbol{\eta}}-\boldsymbol{\eta}\\ \hat{\boldsymbol{\alpha}}-\boldsymbol{\alpha}\end{bmatrix}+\begin{bmatrix}\frac{1}{N}\sum_{i=1}^{N}\boldsymbol{a}_i+C_3\cdot\frac{1}{N_0}\sum_{i=1}^{N_0}\boldsymbol{f}_i\\ \frac{1}{N}\sum_{i=1}^{N}\boldsymbol{b}_i+D_3\cdot\frac{1}{N_0}\sum_{i=1}^{N_0}\boldsymbol{f}_i\end{bmatrix}=\begin{bmatrix}\mathbf{0}\\ \mathbf{0}\end{bmatrix},$$

and finally derive the influence functions for $(\boldsymbol{\eta}^T,\boldsymbol{\alpha}^T)^T$ as

$$\sqrt{N}\begin{bmatrix}\hat{\boldsymbol{\eta}}-\boldsymbol{\eta}\\ \hat{\boldsymbol{\alpha}}-\boldsymbol{\alpha}\end{bmatrix}=-M^{-1}\begin{bmatrix}\sum_y\frac{1}{\sqrt{N_y}}\sum_{i=1}^{N_y}p_y^{1/2}\boldsymbol{a}_i+\frac{1}{\sqrt{N_0}}\sum_{i=1}^{N_0}p_0^{-1/2}C_3\boldsymbol{f}_i\\ \frac{1}{\sqrt{N}}\sum_{i=1}^{N}\boldsymbol{b}_i+\frac{1}{\sqrt{N_0}}\sum_{i=1}^{N_0}p_0^{-1/2}D_3\boldsymbol{f}_i\end{bmatrix}.$$

Then we define the covariance-variance matrix $V$ as

$$V=\begin{bmatrix}V_{11} & V_{12}\\ V_{12}^T & V_{22}\end{bmatrix},$$

where

$$\begin{aligned}V_{11}&=\mathrm{cov}(\boldsymbol{a}_i)+p_0^{-1}\mathrm{cov}_0(C_3\boldsymbol{f}_i)+\mathrm{cov}_0(\boldsymbol{a}_i,C_3\boldsymbol{f}_i)+\mathrm{cov}_0(C_3\boldsymbol{f}_i,\boldsymbol{a}_i),\\ V_{22}&=\mathrm{cov}(\boldsymbol{b}_i)+p_0^{-1}\mathrm{cov}_0(D_3\boldsymbol{f}_i)+\mathrm{cov}_0(\boldsymbol{b}_i,D_3\boldsymbol{f}_i)+\mathrm{cov}_0(D_3\boldsymbol{f}_i,\boldsymbol{b}_i),\\ V_{12}&=\mathrm{cov}(\boldsymbol{a}_i,\boldsymbol{b}_i)+\mathrm{cov}_0(C_3\boldsymbol{f}_i,\boldsymbol{b}_i)+\mathrm{cov}_0(\boldsymbol{a}_i,D_3\boldsymbol{f}_i)+p_0^{-1}\mathrm{cov}_0(C_3\boldsymbol{f}_i,D_3\boldsymbol{f}_i),\end{aligned}$$

and covariance $\mathrm{cov}_0$ is taken with respect to the joint probability of $(\boldsymbol{X},G)$ within controls, i.e., $\mathrm{P}(\boldsymbol{X},G|Y=0)$, and cov is taken with respect to the joint probability $\mathrm{P}(\boldsymbol{X},G)$ in the full case-control sample. Covariance-variance matrices $\mathrm{cov}_0$ and cov can be consistently empirically estimated using corresponding covariances within controls and in the full sample, respectively. Suppose that the true values of $\boldsymbol{\eta}$ and $\boldsymbol{\alpha}$ lie inside a compact space, and that component of $(\boldsymbol{X},G)$ are bounded. Under regularity conditions, $(\hat{\boldsymbol{\eta}}^T,\hat{\boldsymbol{\alpha}}^T)^T$ is consistently and asymptotically normally distributed with

$$\sqrt{N}\begin{bmatrix}\hat{\boldsymbol{\eta}}-\boldsymbol{\eta}\\ \hat{\boldsymbol{\alpha}}-\boldsymbol{\alpha}\end{bmatrix}\xrightarrow{D}N\left(\begin{bmatrix}\mathbf{0}\\ \mathbf{0}\end{bmatrix},M^{-1}V(M^{-1})^T\right).$$

## References

[1] A W van der Vaart. *Asymptotic statistics*. Cambridge University Press, 1998.

Table 1: Distribution of children's genotypes ($G^c$) conditional on parents' genotypes ($G$ and $G^s$) under the assumption of Mendelian inheritance.

| $G$ | $G^s$ | $G^c$ | | |
|---|---|---|---|---|
| | | 0 | 1 | 2 |
| 0 | 0 | 1 | 0 | 0 |
| 0 | 1 | 0.5 | 0.5 | 0 |
| 0 | 2 | 0 | 1 | 0 |
| 1 | 0 | 0.5 | 0.5 | 0 |
| 1 | 1 | 0.25 | 0.5 | 0.25 |
| 1 | 2 | 0 | 0.5 | 0.5 |
| 2 | 0 | 0 | 1 | 0 |
| 2 | 1 | 0 | 0.5 | 0.5 |
| 2 | 2 | 0 | 0 | 1 |

Table 2: The estimated log odds ratios in the missingness model using the family-supplemented weighted empirical likelihood method. The prevalence is 0.03 and the minor allele frequency is 0.2. The true values of $(\alpha_3, \alpha_4, \alpha_5)$ in the three missingness models are: weak $= (0.182, 0.405, 0.405)$, strong $= (0.405, 0.405, 0.405)$, and non-differential (ND) $= (0.405, 0, 0)$. The true values of $\alpha_0$ are 1.21, 1.13, and 1.14 in model weak, strong, and ND when the genotype availability is 0.8 and are 0.22, 0.14, 0.16 when the genotype availability is 0.6. The mean asymptotic standard error ("asym") and empirical standard error ("emp") of $\hat{\boldsymbol{\alpha}}$ were calculated based on 1000 simulations.

| $P(R=1)$ | $e^{\beta_2}$ | missing | $\hat{\alpha}_0$ | $\hat{\alpha}_1$ | $\hat{\alpha}_2$ |
|---|---|---|---|---|---|
| 0.8 | 1.2 | weak | 1.213 (0.115/0.114) | -0.513 (0.162/0.165) | 0.180 (0.119/0.116) |
| | | strong | 1.123 (0.113/0.113) | -0.506 (0.160/0.156) | 0.192 (0.119/0.116) |
| | | ND | 1.139 (0.113/0.113) | -0.512 (0.156/0.162) | 0.190 (0.120/0.117) |
| | 1.5 | weak | 1.211 (0.114/0.115) | -0.509 (0.165/0.162) | 0.180 (0.119/0.118) |
| | | strong | 1.138 (0.113/0.117) | -0.519 (0.163/0.165) | 0.175 (0.119/0.119) |
| | | ND | 1.140 (0.113/0.116) | -0.508 (0.158/0.156) | 0.186 (0.120/0.120) |
| 0.6 | 1.2 | weak | 0.224 (0.092/0.094) | -0.517 (0.136/0.136) | 0.182 (0.097/0.097) |
| | | strong | 0.135 (0.092/0.094) | -0.509 (0.137/0.140) | 0.188 (0.098/0.097) |
| | | ND | 0.160 (0.092/0.095) | -0.514 (0.133/0.138) | 0.180 (0.098/0.097) |
| | 1.5 | weak | 0.223 (0.092/0.093) | -0.511 (0.138 /0.141) | 0.179 (0.097/0.098) |
| | | strong | 0.144 (0.092/0.092) | -0.513 (0.139/0.133) | 0.180 (0.098/0.097) |
| | | ND | 0.159 (0.092/0.094) | -0.506 (0.135/0.137) | 0.187 (0.098/0.099) |

| $P(R=1)$ | $e^{\beta_2}$ | missing | $\hat{\alpha}_3$ | $\hat{\alpha}_4$ | $\hat{\alpha}_5$ |
|---|---|---|---|---|---|
| 0.8 | 1.2 | weak | 0.194 (0.152/0.158) | 0.410 (0.167/0.169) | 0.400 (0.220/0.220) |
| | | strong | 0.423 (0.161/0.161) | 0.401 (0.169/0.162) | 0.408 (0.234/0.222) |
| | | ND | 0.414 (0.162/0.166) | -0.007 (0.161/0.162) | 0.0001 (0.208/0.208) |
| | 1.5 | weak | 0.189 (0.152/0.150) | 0.407 (0.168/0.164) | 0.406 (0.215/0.213) |
| | | strong | 0.408 (0.161/0.164) | 0.418 (0.170/0.163) | 0.407 (0.228/0.230) |
| | | ND | 0.413 (0.162/0.164) | -0.008 (0.161/0.161) | -0.003 (0.204/0.198) |
| 0.6 | 1.2 | weak | 0.181 (0.113/ 0.112) | 0.406 (0.140/0.138) | 0.414 (0.164/0.156) |
| | | strong | 0.411 (0.117/0.120) | 0.404 (0.142/0.141) | 0.412 (0.171/0.168) |
| | | ND | 0.409 (0.118/0.119) | 0.004 (0.139/0.139) | 0.003 (0.157/0.156) |
| | 1.5 | weak | 0.188 (0.113/0.115) | 0.408 (0.140/0.145) | 0.400 (0.160/0.158) |
| | | strong | 0.406 (0.118/0.118) | 0.408 (0.142/0.137) | 0.404 (0.167/0.166) |
| | | ND | 0.408 (0.118/0.120) | -0.008 (0.138/0.144) | -0.005 (0.154/0.149) |

Table 3: The estimated log odds ratios in the association model and the estimated minor allele frequency ($\theta$) using the family-supplemented weighted empirical likelihood method. The prevalence is 0.03 and the minor allele frequency is 0.5. The true values of $(\alpha_3, \alpha_4, \alpha_5)$ in the three missingness models are: weak = $(0.182, 0.405, 0.405)$, strong = $(0.405, 0.405, 0.405)$, and non-differential (ND) = $(0.405, 0, 0)$. The mean asymptotic standard error ("asym"), empirical standard error ("emp"), and coverage probability ("coverage") of $\hat{\beta}_1$, $\hat{\beta}_2$, and $\hat{\theta}$ were calculated based on 1000 simulations.

| $P(R=1)$ | $e^{\beta_2}$ | missing | $\hat{\beta}_1$ | | $\hat{\beta}_2$ | | $\hat{\theta}$ | |
|---|---|---|---|---|---|---|---|---|
| | | | estimate (asy/emp) | coverage | estimate (asy/emp) | coverage | estimate (asy/emp) | coverage |
| 0.8 | 1.2 | weak | 0.182 (0.068/0.061) | 0.978 | 0.183 (0.050/0.051) | 0.942 | 0.498 (0.009/0.009) | 0.960 |
| | | strong | 0.183 (0.068/0.064) | 0.964 | 0.182 (0.049/0.050) | 0.954 | 0.499 (0.009/0.009) | 0.949 |
| | | ND | 0.184 (0.068/0.063) | 0.962 | 0.185 (0.051/0.052) | 0.938 | 0.498 (0.009/0.009) | 0.955 |
| | 1.5 | weak | 0.186 (0.070/0.067) | 0.956 | 0.405 (0.050/0.051) | 0.951 | 0.497 (0.009/0.009) | 0.943 |
| | | strong | 0.180 (0.069/0.065) | 0.965 | 0.403 (0.050/0.047) | 0.961 | 0.497 (0.009/0.009) | 0.939 |
| | | ND | 0.182 (0.069/0.066) | 0.963 | 0.404 (0.052/0.054) | 0.938 | 0.497 (0.009/0.009) | 0.953 |
| 0.6 | 1.2 | weak | 0.182 (0.073/0.061) | 0.983 | 0.183 (0.055/0.056) | 0.953 | 0.498 (0.010/0.010) | 0.965 |
| | | strong | 0.183 (0.073/0.064) | 0.975 | 0.181 (0.056/0.057) | 0.951 | 0.499 (0.010/0.010) | 0.947 |
| | | ND | 0.185 (0.073/0.063) | 0.971 | 0.184 (0.058/0.057) | 0.948 | 0.498 (0.010/0.010) | 0.954 |
| | 1.5 | weak | 0.186 (0.074/0.067) | 0.967 | 0.404 (0.056/0.056) | 0.954 | 0.497 (0.010/0.010) | 0.953 |
| | | strong | 0.180 (0.074/0.066) | 0.975 | 0.402 (0.056/0.055) | 0.952 | 0.497 (0.010/0.010) | 0.949 |
| | | ND | 0.182 (0.074/0.066) | 0.974 | 0.405 (0.059/0.059) | 0.949 | 0.497 (0.010/0.010) | 0.943 |

Table 4: The estimated log odds ratios in the missingness model using the family-supplemented weighted empirical likelihood method. The prevalence is 0.03 and the minor allele frequency is 0.5. The true values of $(\alpha_3, \alpha_4, \alpha_5)$ in the three missingness models are: weak = $(0.182, 0.405, 0.405)$, strong = $(0.405, 0.405, 0.405)$, and non-differential (ND) = $(0.405, 0, 0)$. The true values of $\alpha_0$ are 1.09, 0.89, and 0.93 in model weak, strong, and ND when the genotype availability is 0.8 and are 0.12, -0.10, -0.09 when the genotype availability is 0.6. The mean asymptotic standard error ("asym") and empirical standard error ("emp") of $\hat{\boldsymbol{\alpha}}$ were calculated based on 1000 simulations.

| P$(R = 1)$ | $e^{\beta_2}$ | missing | $\hat{\alpha}_0$ | $\hat{\alpha}_1$ | $\hat{\alpha}_2$ |
|---|---|---|---|---|---|
| 0.8 | 1.2 | weak | 1.097 (0.144/0.148) | -0.515 (0.211/0.212) | 0.180 (0.113/0.111) |
| | | strong | 0.892 (0.140/0.143) | -0.512 (0.207/0.201) | 0.182 (0.114/0.113) |
| | | ND | 0.926 (0.142/0.148) | -0.504 (0.195/0.200) | 0.187 (0.116/0.113) |
| | 1.5 | weak | 1.090 (0.144/0.149) | -0.514 (0.220/0.223) | 0.184 (0.113/0.108) |
| | | strong | 0.891 (0.140/0.146) | -0.508 (0.216/0.221) | 0.181 (0.114/0.116) |
| | | ND | 0.931 (0.142/0.149) | -0.506 (0.201/0.210) | 0.184 (0.116/0.119) |
| 0.6 | 1.2 | weak | 0.120 (0.114/0.120) | -0.511 (0.171/0.172) | 0.183 (0.093/ 0.093) |
| | | strong | -0.098 (0.113/0.114) | -0.510 (0.172/0.171) | 0.182 (0.094/0.093) |
| | | ND | -0.095 (0.114/0.115) | -0.502 (0.164/0.164) | 0.188 (0.094/0.093) |
| | 1.5 | weak | 0.119 (0.114/ 0.111) | -0.510 (0.177/0.173) | 0.185 (0.093/0.091) |
| | | strong | -0.096 (0.113/0.115) | -0.517 (0.178/0.178) | 0.181 (0.094/0.093) |
| | | ND | -0.090 (0.113/0.113) | -0.504 (0.169/0.166) | 0.185 (0.094/0.093) |

| P$(R = 1)$ | $e^{\beta_2}$ | missing | $\hat{\alpha}_3$ | $\hat{\alpha}_4$ | $\hat{\alpha}_5$ |
|---|---|---|---|---|---|
| 0.8 | 1.2 | weak | 0.179 (0.120/0.122) | 0.415 (0.165/0.167) | 0.403 (0.179/0.175) |
| | | strong | 0.404 (0.121/0.123) | 0.407 (0.168/0.165) | 0.407 (0.183/0.175) |
| | | ND | 0.410 (0.124/0.131) | 0.001 (0.155/0.154) | -0.007 (0.163/0.168) |
| | 1.5 | weak | 0.184 (0.120/0.123) | 0.409 (0.167/0.164) | 0.407 (0.181/0.176) |
| | | strong | 0.408 (0.122/0.127) | 0.405 (0.169/0.172) | 0.405 (0.185/0.187) |
| | | ND | 0.409 (0.124/0.126) | 0.001 (0.156/0.159) | -0.005 (0.164/0.167) |
| 0.6 | 1.2 | weak | 0.182 (0.090/0.094) | 0.406 (0.136/0.135) | 0.405 (0.135/0.133) |
| | | strong | 0.404 (0.091/0.094) | 0.408 (0.139/0.135) | 0.407 (0.139/0.139) |
| | | ND | 0.408 (0.092/0.094) | -0.006 (0.133/0.133) | -0.004 (0.127/0.126) |
| | 1.5 | weak | 0.182 (0.090/0.090) | 0.400 (0.136/0.138) | 0.409 (0.136/0.131) |
| | | strong | 0.402 (0.092/0.093) | 0.407 (0.139/0.141) | 0.413 (0.140/0.138) |
| | | ND | 0.405 (0.092/0.092) | -0.007 (0.133/0.128) | -0.004 (0.127/0.125) |

Table 5: The bias and mean squared error (MSE) of the estimated log odds ratios in the association model and the estimated minor allele frequency ($\theta$) based on 1000 simulations. The prevalence is 0.03 and the minor allele frequency is 0.5. The true values of $(\alpha_3, \alpha_4, \alpha_5)$ in the three missingness models are: weak = $(0.182, 0.405, 0.405)$, strong = $(0.405, 0.405, 0.405)$, and non-differential (ND) = $(0.405, 0, 0)$. In each of the 12 settings, true values and estimates of coefficients $\beta_1$, $\beta_2$ and $\theta$ are presented in this order in the magnitude of $10^{-3}$.

| Model | | | | MCAR | | FS-WEL | |
|---|---|---|---|---|---|---|---|
| P$(R=1)$ | $e^{\beta_2}$ | Missing | True | Bias | MSE | Bias | MSE |
| 0.8 | 1.2 | weak | 182 | 72.324 | 10.124 | 0.033 | 3.739 |
| | | | 182 | 67.926 | 7.017 | 1.042 | 2.566 |
| | | | 500 | 6.948 | 0.128 | -1.725 | 0.080 |
| | | strong | 182 | 67.882 | 9.920 | 0.288 | 4.083 |
| | | | 182 | 62.074 | 6.475 | -0.631 | 2.506 |
| | | | 500 | 18.470 | 0.421 | -1.190 | 0.083 |
| | | ND | 182 | 18.951 | 5.832 | 2.062 | 3.984 |
| | | | 182 | 37.357 | 4.048 | 2.326 | 2.737 |
| | | | 500 | 17.588 | 0.386 | -1.636 | 0.083 |
| | 1.5 | weak | 182 | 72.487 | 10.654 | 3.643 | 4.445 |
| | | | 405 | 66.778 | 7.044 | -0.168 | 2.595 |
| | | | 500 | 6.040 | 0.111 | -2.865 | 0.090 |
| | | strong | 182 | 64.075 | 9.092 | -2.146 | 4.196 |
| | | | 405 | 59.557 | 6.001 | -2.480 | 2.258 |
| | | | 500 | 16.818 | 0.360 | -2.908 | 0.088 |
| | | ND | 182 | 15.933 | 5.963 | -0.193 | 4.409 |
| | | | 405 | 34.628 | 4.129 | -1.024 | 2.946 |
| | | | 500 | 16.351 | 0.343 | -2.841 | 0.086 |
| 0.6 | 1.2 | weak | 182 | 138.307 | 25.742 | 0.090 | 3.746 |
| | | | 182 | 133.852 | 21.147 | 0.527 | 3.087 |
| | | | 500 | 15.832 | 0.360 | -1.699 | 0.098 |
| | | strong | 182 | 131.333 | 23.961 | 0.624 | 4.102 |
| | | | 182 | 120.563 | 18.015 | -1.693 | 3.245 |
| | | | 500 | 38.113 | 1.558 | -1.086 | 0.105 |
| | | ND | 182 | 22.227 | 8.218 | 2.412 | 3.999 |
| | | | 182 | 51.096 | 6.351 | 2.069 | 3.282 |
| | | | 500 | 37.579 | 1.514 | -1.724 | 0.101 |
| | 1.5 | weak | 182 | 136.611 | 25.988 | 3.697 | 4.506 |
| | | | 405 | 131.872 | 20.655 | -1.853 | 3.127 |
| | | | 500 | 14.835 | 0.322 | -2.625 | 0.110 |
| | | strong | 182 | 126.493 | 22.998 | -2.285 | 4.301 |
| | | | 405 | 120.704 | 17.906 | -3.164 | 2.981 |
| | | | 500 | 36.126 | 1.408 | -2.717 | 0.107 |
| | | ND | 182 | 19.535 | 8.242 | 0.092 | 4.395 |
| | | | 405 | 48.261 | 6.026 | -0.392 | 3.442 |
| | | | 500 | 36.311 | 1.412 | -2.771 | 0.109 |

MCAR: missing completely at random; FS-WEL: family-supplemented weighted empirical likelihood method.

Table 6: The estimated log odds ratios in the association model and the estimated minor allele frequency ($\theta$) using the family-supplemented weighted empirical likelihood method. The prevalence is 0.10 and the minor allele frequency is 0.5. The true values of $(\alpha_3, \alpha_4, \alpha_5)$ in the three missingness models are: weak = $(0.182, 0.405, 0.405)$, strong = $(0.405, 0.405, 0.405)$, and non-differential (ND) = $(0.405, 0, 0)$. The mean asymptotic standard error ("asym"), empirical standard error ("emp"), and coverage probability ("coverage") of $\hat{\beta}_1$, $\hat{\beta}_2$, and $\hat{\theta}$ were calculated based on 1000 simulations.

| P$(R=1)$ | $e^{\alpha_2}$ | missing | $\hat{\beta}_1$ | | $\hat{\beta}_2$ | | $\hat{\theta}$ | |
|---|---|---|---|---|---|---|---|---|
| | | | estimate (asy/emp) | coverage | estimate (asy/emp) | coverage | estimate (asy/emp) | coverage |
| 0.8 | 1.2 | weak | 0.181 (0.068/0.066) | 0.958 | 0.181 (0.049/0.052) | 0.939 | 0.495 (0.0093/0.0090) | 0.915 |
| | | strong | 0.181 (0.068/0.066) | 0.948 | 0.182 (0.049/0.052) | 0.933 | 0.495 (0.0093/0.0092) | 0.927 |
| | | ND | 0.183 (0.068/0.063) | 0.966 | 0.185 (0.051/0.053) | 0.933 | 0.495 (0.0092/0.0091) | 0.931 |
| | 1.5 | weak | 0.182 (0.070/0.065) | 0.963 | 0.402 (0.050/0.050) | 0.954 | 0.490 (0.0093/0.0090) | 0.824 |
| | | strong | 0.181 (0.070/0.063) | 0.968 | 0.406 (0.050/0.051) | 0.943 | 0.490 (0.0093/0.0091) | 0.802 |
| | | ND | 0.186 (0.069/0.066) | 0.959 | 0.402 (0.051/0.051) | 0.954 | 0.490 (0.0092/0.0087) | 0.818 |
| 0.6 | 1.2 | weak | 0.181 (0.073/0.066) | 0.960 | 0.181 (0.056/0.057) | 0.939 | 0.495 (0.0105/0.0101) | 0.925 |
| | | strong | 0.180 (0.073/0.066) | 0.966 | 0.181 (0.056/0.058) | 0.931 | 0.495 (0.0105/0.0105) | 0.930 |
| | | ND | 0.183 (0.072/0.064) | 0.973 | 0.184 (0.058/0.059) | 0.941 | 0.495 (0.0104/0.0101) | 0.930 |
| | 1.5 | weak | 0.182 (0.074/0.066) | 0.975 | 0.401 (0.056/0.056) | 0.954 | 0.490 (0.0105/0.0099) | 0.864 |
| | | strong | 0.181 (0.074/0.063) | 0.977 | 0.406 (0.056/0.056) | 0.949 | 0.490 (0.0105/0.0101) | 0.853 |
| | | ND | 0.186 (0.074/0.066) | 0.968 | 0.402 (0.058/0.057) | 0.962 | 0.490 (0.0104/0.0097) | 0.851 |

Table 7: The estimated log odds ratios in the missingness model using the family-supplemented weighted empirical likelihood method. The prevalence is 0.10 and the minor allele frequency is 0.5. The true values of $(\alpha_3, \alpha_4, \alpha_5)$ in the three missingness models are: weak = $(0.182, 0.405, 0.405)$, strong = $(0.405, 0.405, 0.405)$, and non-differential (ND) = $(0.405, 0, 0)$. The true values of $\alpha_0$ are 1.09, 0.89, and 0.95 in model weak, strong, and ND when the genotype availability is 0.8 and are 0.10, -0.11, -0.045 when the genotype availability is 0.6. The mean asymptotic standard error ("asym") and empirical standard error ("emp") of $\hat{\boldsymbol{\alpha}}$ were calculated based on 1000 simulations.

| $\mathrm{P}(R=1)$ | $e^{\beta_2}$ | missing | $\hat{\alpha}_0$ | $\hat{\alpha}_1$ | $\hat{\alpha}_2$ |
|---|---|---|---|---|---|
| 0.8 | 1.2 | weak | 1.089 (0.143/0.142) | -0.512 (0.210/0.206) | 0.178 (0.113/0.115) |
| | | strong | 0.883 (0.140/0.137) | -0.508 (0.206/0.197) | 0.190 (0.114/0.113) |
| | | ND | 0.950 (0.142/0.142) | -0.511 (0.195/0.196) | 0.180 (0.116/0.115) |
| | 1.5 | weak | 1.090 (0.143/0.147) | -0.515 (0.219/0.223) | 0.189 (0.113/0.115) |
| | | strong | 0.891 (0.140/0.137) | -0.520 (0.215/0.218) | 0.185 (0.114/0.114) |
| | | ND | 0.946 (0.142/0.149) | -0.506 (0.201/0.203) | 0.185 (0.116/0.120) |
| 0.6 | 1.2 | weak | 0.100 (0.113/0.115) | -0.519 (0.170/0.177) | 0.184 (0.093/0.091) |
| | | strong | -0.108 (0.113/0.113) | -0.520 (0.171/0.170) | 0.180 (0.094/0.093) |
| | | ND | -0.045 (0.114/0.116) | -0.511 (0.164/0.160) | 0.180 (0.095/0.091) |
| | 1.5 | weak | 0.102 (0.113/0.122) | -0.519 (0.175/0.184) | 0.181 (0.093/0.097) |
| | | strong | -0.111 (0.113/0.115) | -0.507 (0.177/0.177) | 0.185 (0.094/0.095) |
| | | ND | -0.047 (0.113/0.116) | -0.511 (0.168 /0.169) | 0.181 (0.095/0.097) |

| $\mathrm{P}(R=1)$ | $e^{\beta_2}$ | missing | $\hat{\alpha}_3$ | $\hat{\alpha}_4$ | $\hat{\alpha}_5$ |
|---|---|---|---|---|---|
| 0.8 | 1.2 | weak | 0.187 (0.120/0.120) | 0.412 (0.165/0.164) | 0.407 (0.179/0.179) |
| | | strong | 0.417 (0.122/0.123) | 0.404 (0.168/0.167) | 0.397 (0.184/0.177) |
| | | ND | 0.410 (0.125/0.127) | 0.002 (0.156/0.154) | -0.002 (0.164/0.166) |
| | 1.5 | weak | 0.184 (0.121/0.124) | 0.403 (0.166/0.168) | 0.411 (0.182/0.186) |
| | | strong | 0.408 (0.123/0.124) | 0.407 (0.169/0.176) | 0.415 (0.186/0.185) |
| | | ND | 0.411 (0.125/0.129) | 0.003 (0.156/0.161) | -0.005 (0.166/0.168) |
| 0.6 | 1.2 | weak | 0.180 (0.089/0.093) | 0.411 (0.136/0.133) | 0.414 (0.135/0.143) |
| | | strong | 0.409 (0.091/0.096) | 0.414 (0.138/0.136) | 0.407 (0.139/0.139) |
| | | ND | 0.407 (0.093/0.095) | 0.004 (0.133/0.129) | -0.001 (0.128/0.129) |
| | 1.5 | weak | 0.184 (0.090/0.096) | 0.412 (0.136/0.137) | 0.408 (0.136/0.144) |
| | | strong | 0.406 (0.092/0.095) | 0.404 (0.138/0.137) | 0.406 (0.140/0.139) |
| | | ND | 0.408 (0.093/0.095) | -0.001 (0.133/0.139) | 0.002 (0.128/0.126) |

Table 8: The bias and mean squared error (MSE) in the association model based on 1000 simulations. The prevalence is 0.10 and the minor allele frequency is 0.5. The true values of $(\alpha_3, \alpha_4, \alpha_5)$ in the three missingness models are: weak = $(0.182, 0.405, 0.405)$, strong = $(0.405, 0.405, 0.405)$, and non-differential (ND) = $(0.405, 0, 0)$. In each of the 12 settings, true values and estimates of coefficients $\beta_1$, $\beta_2$ and $\theta$ are presented in this order in the magnitude of $10^{-3}$.

| Model | | | | MCAR | | FS-WEL | |
|---|---|---|---|---|---|---|---|
| $P(R=1)$ | $e^{\beta_2}$ | Missing | True | Bias | MSE | Bias | MSE |
| 0.8 | 1.2 | weak | 182 | 70.375 | 10.634 | -1.484 | 4.325 |
| | | | 182 | 66.544 | 6.952 | -0.919 | 2.669 |
| | | | 500 | 4.121 | 0.091 | -4.955 | 0.105 |
| | | strong | 182 | 67.080 | 9.962 | -1.729 | 4.412 |
| | | | 182 | 61.865 | 6.395 | -0.154 | 2.697 |
| | | | 500 | 15.142 | 0.307 | -4.934 | 0.109 |
| | | ND | 182 | 16.610 | 5.638 | 0.217 | 4.015 |
| | | | 182 | 38.474 | 4.203 | 2.395 | 2.856 |
| | | | 500 | 13.799 | 0.274 | -5.146 | 0.109 |
| | 1.5 | weak | 182 | 69.026 | 10.241 | -0.304 | 4.260 |
| | | | 405 | 65.704 | 6.753 | -3.477 | 2.486 |
| | | | 500 | -0.985 | 0.077 | -9.807 | 0.176 |
| | | strong | 182 | 66.699 | 9.686 | -1.199 | 3.995 |
| | | | 405 | 66.490 | 7.217 | 0.892 | 2.587 |
| | | | 500 | 9.217 | 0.165 | -10.431 | 0.192 |
| | | ND | 182 | 21.966 | 6.250 | 3.630 | 4.406 |
| | | | 405 | 33.733 | 3.781 | -3.053 | 2.614 |
| | | | 500 | 9.023 | 0.161 | -9.923 | 0.175 |
| 0.6 | 1.2 | weak | 182 | 140.213 | 26.990 | -1.713 | 4.398 |
| | | | 182 | 136.738 | 22.004 | -1.427 | 3.288 |
| | | | 500 | 12.732 | 0.257 | -4.788 | 0.124 |
| | | strong | 182 | 134.456 | 25.394 | -2.097 | 4.407 |
| | | | 182 | 122.709 | 18.591 | -1.605 | 3.365 |
| | | | 500 | 35.114 | 1.338 | -4.597 | 0.131 |
| | | ND | 182 | 24.989 | 7.967 | 0.230 | 4.071 |
| | | | 182 | 51.520 | 6.623 | 1.195 | 3.494 |
| | | | 500 | 33.260 | 1.211 | -4.896 | 0.127 |
| | 1.5 | weak | 182 | 140.514 | 27.382 | -0.416 | 4.310 |
| | | | 405 | 132.061 | 20.802 | -4.365 | 3.206 |
| | | | 500 | 8.218 | 0.169 | -9.628 | 0.191 |
| | | strong | 182 | 128.610 | 23.314 | -1.694 | 3.977 |
| | | | 405 | 124.718 | 18.915 | 0.635 | 3.159 |
| | | | 500 | 29.057 | 0.946 | -10.227 | 0.207 |
| | | ND | 182 | 26.604 | 8.726 | 3.285 | 4.425 |
| | | | 405 | 49.575 | 6.249 | -3.828 | 3.214 |
| | | | 500 | 28.185 | 0.898 | -9.964 | 0.193 |

MCAR: missing completely at random; FS-WEL: family-supplemented weighted empirical likelihood method.

Table 9: The estimated log odds ratios in the association model and the estimated minor allele frequency ($\theta$) using the family-supplemented weighted empirical likelihood method when missingness is completely at random. The prevalence is 0.05. The mean asymptotic standard error ("asym"), empirical standard error ("emp"), and coverage probability ("coverage") were calculated based on 1000 simulations.

| MAF | P($R=1$) | $e^{\beta_2}$ | $\hat{\beta}_1$ | | $\hat{\beta}_2$ | | $\hat{\theta}$ | |
|---|---|---|---|---|---|---|---|---|
| | | | estimate (asy/emp) | coverage | estimate (asy/emp) | coverage | estimate (asy/emp) | coverage |
| 0.2 | 0.8 | 1.2 | 0.181 (0.071/0.068) | 0.969 | 0.177 (0.060/0.061) | 0.950 | 0.200 (0.007/0.007) | 0.945 |
| | | 1.5 | 0.182 (0.074/0.067) | 0.980 | 0.407 (0.058/0.060) | 0.943 | 0.198 (0.007/0.007) | 0.948 |
| | | 1.2 | 0.183 (0.076/0.068) | 0.976 | 0.180 (0.067/0.066) | 0.949 | 0.200 (0.008/0.008) | 0.947 |
| | | 1.5 | 0.187 (0.079/0.071) | 0.970 | 0.402 (0.065/0.067) | 0.938 | 0.198 (0.008/0.008) | 0.946 |
| 0.5 | 0.6 | 1.2 | 0.184 (0.068/0.067) | 0.955 | 0.182 (0.050/0.051) | 0.950 | 0.499 (0.009/0.009) | 0.949 |
| | | 1.5 | 0.181 (0.070/0.066) | 0.967 | 0.404 (0.051/0.050) | 0.955 | 0.496 (0.009/0.009) | 0.934 |
| | | 1.2 | 0.181 (0.073/0.066) | 0.969 | 0.181 (0.056/0.058) | 0.937 | 0.499 (0.010/0.010) | 0.945 |
| | | 1.5 | 0.181 (0.075/0.067) | 0.972 | 0.405 (0.057/0.057) | 0.948 | 0.497 (0.010/0.010) | 0.950 |

Table 10: The bias and mean squared error (MSE) in the association model and the estimated minor allele frequency ($\theta$) based on 1000 simulations when missingness is completely at random. The prevalence is 0.05. In each of the 12 settings, true values and estimates of coefficients $\beta_1$, $\beta_2$ and $\theta$ are presented in this order in the magnitude of $10^{-3}$.

| Model | | | | MCAR | | FS-WEL | |
|---|---|---|---|---|---|---|---|
| MAF | P($R = 1$) | $e^{\beta_2}$ | True | Bias | MSE | Bias | MSE |
| 0.2 | 0.8 | 1.2 | 182 | -1.202 | 5.488 | -1.644 | 4.565 |
| | | | 182 | -4.010 | 3.870 | -5.498 | 3.802 |
| | | | 200 | -0.196 | 0.049 | -0.364 | 0.050 |
| | | 1.5 | 182 | 1.735 | 5.587 | -0.491 | 4.490 |
| | | | 405 | 3.370 | 3.749 | 1.550 | 3.650 |
| | | | 200 | -2.277 | 0.055 | -2.257 | 0.055 |
| | 0.6 | 1.2 | 182 | 1.446 | 7.926 | 0.512 | 4.682 |
| | | | 182 | 0.041 | 4.805 | -2.439 | 4.421 |
| | | | 200 | -0.783 | 0.069 | -0.368 | 0.061 |
| | | 1.5 | 182 | 4.636 | 7.570 | 4.536 | 4.991 |
| | | | 405 | -3.264 | 4.828 | -3.064 | 4.443 |
| | | | 200 | -1.715 | 0.070 | -1.724 | 0.064 |
| 0.5 | 0.8 | 1.2 | 182 | 0.640 | 5.752 | -0.515 | 4.532 |
| | | | 182 | 0.493 | 2.678 | -0.116 | 2.621 |
| | | | 500 | -1.264 | 0.084 | -1.371 | 0.084 |
| | | 1.5 | 182 | -0.665 | 5.303 | -0.892 | 4.311 |
| | | | 405 | -1.613 | 2.452 | -0.982 | 2.506 |
| | | | 500 | -3.569 | 0.090 | -3.754 | 0.095 |
| | 0.6 | 1.2 | 182 | 0.039 | 7.220 | -0.866 | 4.327 |
| | | | 182 | 0.742 | 3.518 | -1.337 | 3.370 |
| | | | 500 | -1.557 | 0.110 | -1.220 | 0.109 |
| | | 1.5 | 182 | 0.804 | 7.074 | -0.860 | 4.541 |
| | | | 405 | 2.450 | 3.519 | -0.475 | 3.245 |
| | | | 500 | -3.412 | 0.113 | -3.097 | 0.106 |

MCAR: missing completely at random; FS-WEL: family-supplemented weighted empirical likelihood method.

Table 11: Distribution of covariates in the Two Sister Study.

| | Case | Control |
|---|---|---|
| $X_1 \leq 24$ | 110(21%) | 229(25%) |
| $(24, 30]$ | 143(28%) | 294(32%) |
| $> 30$ | 110(21%) | 160(17%) |
| NL | 158(30%) | 241(26%) |
| $X_2 \leq 12$ | 238(46%) | 386(42%) |
| $(12, 14)$ | 171(33%) | 295(32%) |
| $\geq 14$ | 112(21%) | 243(26%) |
| Total | 521(36%) | 924(64%) |

NL: nulliparous

Table 12: Estimated log odds ratio parameters and the asymptotic standard errors (asy) in the association model of the Two Sister Study

| | Association Model | | | | Missingness Model |
|---|---|---|---|---|---|
| Model | FS-WEL (asy) | $p$-value | Naive (asy) | $p$-value | $p$-value |
| rs8051542 | 0.257 (0.237) | 0.139 | 0.215 (0.186) | 0.124 | 0.358 |
| $X_1$ (24, 30] | -0.081 (0.319) | 0.400 | -0.092 (0.300) | 0.379 | 0.061 |
| $> 30$ | 0.641 (0.341) | 0.030 | 0.636 (0.341) | 0.031 | 0.024 |
| NL | 0.415 (0.435) | 0.170 | 0.354 (0.277) | 0.101 | 0.187 |
| $X_2$ (12, 14) | 0.248 (0.203) | 0.112 | 0.381 (0.187) | 0.021 | 0.107 |
| $\leq 12$ | 0.339 (0.228) | 0.069 | 0.442 (0.176) | 0.006 | 0.125 |
| Interaction (24, 30] | 0.243 (0.279) | 0.192 | 0.286 (0.266) | 0.141 | |
| $> 30$ | -0.039 (0.311) | 0.451 | 0.037 (0.317) | 0.453 | |
| NL | -0.206 (0.416) | 0.310 | -0.147 (0.254) | 0.281 | |
| MAF | 0.401 (0.011) | | 0.390 (0.026) | | |
| rs8046979 | -0.285 (0.228) | 0.106 | -0.282 (0.189) | 0.068 | 0.410 |
| $X_1$ (24, 30] | 0.263 (0.332) | 0.214 | 0.264 (0.329) | 0.211 | 0.059 |
| $> 30$ | 0.797 (0.419) | 0.028 | 0.777 (0.388) | 0.022 | 0.024 |
| NL | -0.373 (0.466) | 0.211 | -0.348 (0.311) | 0.131 | 0.199 |
| $X_2$ (12, 14) | 0.368 (0.210) | 0.040 | 0.401 (0.187) | 0.016 | 0.101 |
| $\leq 12$ | 0.388 (0.240) | 0.053 | 0.463 (0.176) | 0.004 | 0.119 |
| Interaction (24, 30] | -0.114 (0.274) | 0.339 | -0.095 (0.270) | 0.362 | |
| $> 30$ | -0.196 (0.348) | 0.286 | -0.105 (0.305) | 0.365 | |
| NL | 0.667 (0.508) | 0.095 | 0.632 (0.261) | 0.008 | |
| MAF | 0.498 (0.011) | | 0.486 (0.027) | | |
| rs43143 | -0.051 (0.254) | 0.421 | -0.028 (0.185) | 0.440 | 0.470 |
| $X_1$ (24, 30] | 0.305 (0.304) | 0.158 | 0.345 (0.293) | 0.120 | 0.060 |
| $> 30$ | 0.714 (0.364) | 0.025 | 0.778 (0.343) | 0.012 | 0.024 |
| NL | 0.168 (0.535) | 0.377 | 0.194 (0.299) | 0.259 | 0.186 |
| $X_2$ (12, 14) | 0.283 (0.199) | 0.078 | 0.393 (0.186) | 0.017 | 0.103 |
| $\leq 12$ | 0.373 (0.227) | 0.051 | 0.438 (0.175) | 0.006 | 0.120 |
| Interaction (24, 30] | -0.113 (0.272) | 0.338 | -0.187 (0.264) | 0.240 | |
| $> 30$ | -0.097 (0.324) | 0.382 | -0.118 (0.295) | 0.344 | |
| NL | 0.085 (0.454) | 0.426 | 0.045 (0.253) | 0.430 | |
| MAF | 0.440 (0.011) | | 0.446 (0.027) | | |

NL: nulliparous
